# Supplementary material for: Urgency Annotations for Alternating Choices
Source: arXiv:2305.02967 source file (2023-10-20)
Supplement: Supplementary file 1 [file appendix.tex]

\newpage 

\section{Appendix}
\rfm{BEGIN: Moved this here, check whether notation is consistent:}
\svdw{Obsolete: \rabsbotname{} gone, right?}
$\textbf{\rabsbotname:}$ 
For all objectives $\objective\subseteq\analph^{*}$, 
and any for any $\awordpp, \awordppp\in\analph^{*}$ we have 
that $\awordpp\appl\aword\appl\bot\appl\awordppp\not\in\objective$,
$\awordpp\appl\bot\appl\awordppp\not\in\objective$, and 
$\awordpp\appl\bot\appl\aword\appl\awordppp\not\in\objective$.
So $\aword\appl\bot\sgeq{\objective}\bot\sgeq{\objective}
\bot\appl\aword$.
Since \labelcref{axiom:eqmap} is sound, we have 
$\aword\appl\bot\speccongeq{\objective}\bot\speccongeq{\objective}
\bot\appl\aword$ for all $\objective\subseteq\analph^{*}$.
This is equivalent to $\aword\appl\bot\congeq\bot\congeq
\bot\appl\aword$.
\rfm{END: Moved this here.}

\todo{UNDER VERY HEAVY CONSTRUCTION AND 
OUTDATED. WON'T GET BETTER UNTIL 
THE PAPER IS IN AN OK STATE}
We show that there is a proof for the following rules: 
$$ 
    \axdef{(X2)}{\atermp\axleq\aterm, \anurg=\urgencyof{\aterm}}
    {\aterm\axeq\aterm\echoicen{\anurg}\atermp}
    \qquad
    \axdef{(X3)}{\aterm\axleq\atermp, \anurg=\urgencyof{\aterm}}
    {\aterm\axeq\aterm\achoicen{\anurg}\atermp}
$$

We first show (X2). 
Let $\urgencyof{\aterm}=\anurg$.
The direction $\aterm\axleq
\aterm\echoicen{\anurg}\atermp$ is already 
given from \labelcref{axiom:lattice-ord}, so we only need to show the 
remaining direction:
\begin{align*}
    \aterm\echoicen{\anurg}\atermp
    &\axleqper{\labelcref{axiom:lattice-ord}}
    \aterm\echoicen{\anurg}\atermp\echoicen{\anurg}\aterm\\
    &\axleqper{\labelcref{axiom:lattice-mono}}
    \aterm\echoicen{\anurg}\aterm\echoicen{\anurg}\atermp\\
    &=\aterm
\end{align*}

\todo{Show (X3) if we are/will be use it}

Using this, we show the following rule:
$$
\axdef{(X4)}{\anurg=\urgencyof{\aterm}}
{\aterm\axeq\bigEchoiceOf{\anurg}\set{\aterm}}
$$
The direction $\aterm\axleq\bigEchoiceOf{\anurg}\set{\aterm}$ is 
again already given by \labelcref{axiom:lattice-ord}, so we only prove 
$\bigEchoiceOf{\anurg}\set{\aterm}\axleq\aterm$.

\begin{align*}
    (*)\bot&\axleqper{\labelcref{axiom:least}}\aterm\\
    \aterm&\axeqper{(X2)}\aterm\echoicen{\anurg}\bot
    \text{ using }(*)\\
    &=
    \bigEchoiceOf{\anurg}\set{\aterm, \bot}\\
    \bigEchoiceOf{\anurg}\set{\aterm, \bot}&\axleqper{\labelcref{axiom:lattice-mono}}\aterm
    \text{ letting }\atermpp_{0}=\atermpp_{1}=\aterm,
    \atermppp_{0}=\aterm\text{ and } \atermppp_{1}=\bot\\
\end{align*}

\noindent 
Now we show the Adam-counterpart of \labelcref{axiom:norm}:
$$
\axdef{(NA)}{\anurgp<\anurg}
{
\bigAchoiceOf{\anurgp}\set{\bigPchoiceOf{\anurg}{}{\atermset}}
\axeq\bigAchoiceOf{\anurgp}\set{\bigPchoiceOf{\anurgp}{}{\atermset}
}
}
$$

\begin{align*}
    (*)\bot
    &\axleqper{\labelcref{axiom:least}}
    \bigPchoiceOf{\anurg}{}{\atermset}\\
    \bigAchoiceOf{\anurgp}\set{\bigPchoiceOf{\anurg}{}{\atermset}}
    &\axeqper{(X4)}
    \bigAchoiceOf{\anurgp}\set{\bigPchoiceOf{\anurg}{}{\atermset}}
    \echoicen{\anurgp}
    \bot\\
    &\axeqper{\text{\labelcref{axiom:lattice-dist}}}
    \bigAchoiceOf{\anurgp}\set{(\bigPchoiceOf{\anurg}{}{\atermset})
    \echoicen{\anurgp}\bot}\\
    &\axeqper{\labelcref{axiom:lattice-mono}}
    \bigAchoiceOf{\anurgp}\set{
        \bigEchoiceOf{\anurgp}
        \set{\bigPchoiceOf{\anurg}{}{\atermset}}}\\
    &\axeqper{\labelcref{axiom:norm}}
    \bigAchoiceOf{\anurgp}\set{
        \bigEchoiceOf{\anurgp}
        \set{\bigPchoiceOf{\anurgp}{}{\atermset}}}\\
\end{align*}

\section{Appendix:Completeness}

Let $\objective$ be the specified objective 
in \Cref{Lemma:DomainShattering}.
We show that for all  
$\aword, \awordp\in\analph^{+}$ with $\aword\neq\awordp$,
we can find a $\awordpp\in\analph^{+}$ with
$\aword\appl\awordpp\in\objective$ and 
$\awordp\appl\awordpp\not\in\objective$.
We also need to show that for all $\aword\in\analph^{+}$,
there is a $\awordpp\in\analph^{+}$ with 
$\aword\appl\awordpp\in\alang$ to establish 
the right seperablity of $\aword$ and $\bot$.
The latter proof is straightforward.
Let $\aword\in\analph^{+}$.
If $\analph=\set{\aletter}$, then $\aword=\aletter^{k}$.
Then $\aword\appl\aletter^{4k^{2} - k}\in\objective$.
If $|\analph|>1$, then 
$\aword\appl\aword^{R}\in\objective$.\\

\noindent 
\emph{Proving the existence of $\awordpp$ for $|\analph|=1$:}
We claim that in the case of $\analph=\set{\aletter}$,
$\awordpp=t^{2}-i$ has this property, where 
$\aword=\aletter^{i}$,
$\awordp=\aletter^{j}$, $i\neq j$, and $t=|i - j|+1$.
Suppose $\aletter^{j}\appl\aletter^{t^{2}-i}\in\objective$.
Then, $j+t^{2} - i=k^{2}$ for some $k\in\nat$.
So $j - i=t^{2}-k^{2}$ and thus $|j-i|=|t-k|\cdot|t + k|$.
Since $i\neq j$, we have $t\neq k$ and thus $|t-k|\geq 1$.
We also know that $k>0$ since the words can't be empty.
So $|j-i|=|t-k|\cdot|t + k|<|t|=|j-i|+1$, which is a contradiction.\\

\noindent 
\emph{Proving the existence of $\awordpp$ for $|\analph|>1$:}
We claim that
$\awordpp=\aletter\appl\aword^{R}$ has this property, 
where
$\aletter\neq\aword_{|\awordp|}$ if $|\aword|>|\awordp|$, and
$\aletter\neq\awordp_{|\aword|}$ if $|\awordp|>|\aword|$.
Let $\aletter$ be any terminal from $\analph$ if $|\aword|=|\awordp|$.
Suppose $\awordp\appl\aletter\appl\aword^{R}\in\objective$.
Then it must hold that 
$\awordp\appl\aletter\appl\aword^{R}=\aword\appl\aletter\appl\awordp^{R}$.
If $|\aword|=|\awordp|$,
then $\aword=\awordp$ must hold, which is a contradiction.
Let this be false.
We claim neither of $\aword\appl a$ and $\awordp\appl a$
is the prefix of the other.
If $|\aword|>|\awordp|$, we have that 
$(\awordp\appl\aletter)_{|\awordp|}=\aletter\neq\aword_{|\awordp|}
=(\aword\appl\aletter)_{|\awordp|}$.
If $|\aword|<|\awordp|$, we have that 
$(\aword\appl\aletter)_{|\aword|}=\aletter\neq\awordp_{|\aword|}
=(\awordp\appl\aletter)_{|\aword|}$.

\section{Lower Bound Details}

\noindent\emph{\textbf{Construction:}}
We now formalize our construction, 
starting with the terminal symbols.
The set of terminal symbols $\analph$ consists of assignments 
and assertions of the variables 
$f_{\anurg}\in\states\cup\set{-}$,
$s_{\anurg}\in\states\cup\set{-}$, 
and $c_{\anurg}\in\set{\mathrm{nxt}, \mathrm{sty}}$
for each $0<\anurg\leq\maxurg$.
During each urgency $0<\anurg\leq\maxurg$,
variable $f_{\anurg}$
will keep track of the first MPDG state,
the variable $s_{\anurg}$ will keep track of the 
latest MPDG state, and 
$c_{\anurg}\in\set{\mathrm{nxt}, \mathrm{sty}}$
will be used to enforce the correctness of context switches.
The objective DFA $\adfa$ 
keeps track of the value of these variables.
For each urgency, the DFA also keeps an assertion failure flag
$err_{\anurg}\in\set{\bot, \top}$ for each urgency.
If an assertion failure happens for a variable of 
$\anurg$, then $err_{\anurg}$ is set to $\bot$.
The DFA $\adfa$ accepts if and only if the current state of the 
urgency $1$ is a winning state ($s_{1}\in\goalstates$),
there are no assertion errors ($err_{\anurg}=\top$ for all 
$0<\anurg\leq\maxurg$),
and the latest states are consistent with the first states 
($s_{\anurg+1}=f_{\anurg}$ for all $0<\anurg<\maxurg$).

\ek{Needs to be cleaned up and slightly fixed.}
We now move on to the construction of the terms.
The set of non-terminals is 
$\nonterminals=\set{\ntsymbol{\anurg}\mid 
\stsymbol\in \Gamma, 0<\anurg\leq\maxurg}$.
The representation of an individual stack symbol,
$\wrpsymbol{\anurg}=\bigEchoiceOf{\anurg}\set{\ntsymbol{\anurg}}$,
is the non-terminal wrapped by a trivial urgency $\anurg$ 
choice.
The $\eqmap:\nonterminals\to\terms$ 
is defined below for all 
$\ntsymbol{\anurg}\in\nonterminals$.
We use helper terms to simplify the representation.
Let $\anurg\leq\maxurg$ and $\anurgp<\maxurg$:
\begin{align*}
    \eqmapof{\ntsymbol{\anurg}}
    &=(\assertvar{c_{\anurg}}{\nxt}
    \appl \wrpsymbol{\anurg - 1})
    \echoicen{\anurg}(\assertvar{c_{\anurg}}{\sty}
    \appl \popterm{\stsymbol}{\anurg})\\
    \popterm{\stsymbol}{\anurg}&=\bigEchoiceOf{\anurg}_{\astate\in\states}
    \assertvar{s_{\anurg}}{\astate}\appl
    \encoding{\transitions_{\astate, \stsymbol}}^{\anurg}\qquad
    \encoding{\transitions_{\astate, \stsymbol}}^{\anurg}=
    \bigPchoiceOf{\anurg}_{\atrans\in\transitions_{\astate, \stsymbol}}
    \encoding{\atrans}^{\anurg}_{\stsymbol}\\
    \encoding{\trs{\astate}{\aword:\stsymbol}{\astatep}}^{\anurg}
    _{\stsymbol}
    &=\setvar{s_{\anurg}}{\astatep}\appl
    \aword_{0}^{\anurg}...\aword_{n}^{\anurg}\qquad
    \encoding{\trs{\astate}{\nxt}{\astatep}}^{\maxurg}_{\stsymbol}
    =\wrplsymbol{\anurg}\appl\stacksep\\
    \encoding{\trs{\astate}{\nxt}{\astatep}}^{\anurgp}_{\stsymbol}
    &=\setvar{s_{\anurgp}}{\astatep}\appl\setvar{c_{\anurgp}}{\nxt}\;
    \stacksep=\setvar{c_{1}}{\sty}...\setvar{c_{\maxurg}}{\sty}\\
    \headerurg{\anurg}&=\headerurg{\anurg - 1}\appl
    \bigEchoiceOf{\anurg}_{\astate\in\states}\setvar{f_{\anurg}}{\astate}
    \appl\setvar{s_{\anurg}}{\astate}\\
\end{align*}

\todo{Terminals?}

\ek{A clearer explaination.}
We call a term $\aterm$ $\astate$-state, if
the string $\aword$ acquired by removing all 
outermost actions except terminals has a run in the 
DFA that ends in the
fault-free DFA state that represents an MPDG configuration
with state $\astate$.
Formally, if the resulting DFA has
$err_{\anurg}=\top$ for all $\anurg\leq\maxurg$,
and there is a $\anurg\leq\maxurg$ with
$f_{\anurgp}=s_{\anurgp + 1}$ for all $\anurg<\anurgp<\maxurg$,
$s_{\anurg}=\astate$, and
$f_{\anurgp}=s_{\anurgp}=-$ for all $\anurgp<\anurg$.

\todo{What is a terminal of urgency $\anurg$?}
\todo{$\Pchoice$ owned by the owner of $\astate$}
%
%%\begin{align*}
%    H^{\anurg}&=\bigEchoiceOf{\anurg}_{q\in \states} 
%    \setvar{s_{\anurg}}{\astate}\appl\setvar{f_{\anurg}}{\astate}\\
%    %
%    @&=\setvar{c_{1}}{\mathrm{sty}}...
%    \setvar{c_{\maxurg}}{\mathrm{sty}}\\
%    %
%    Pop_{X}^{\anurg}&=\bigEchoiceOf{\anurg}_{\astate\in\states}
%    \assertvar{s_{\anurg}}{\astate}
%    \appl\encoding{\transitions_{\astate, X}}^{\anurg}\;\;\;
%    %
%    \encoding{\transitions_{\astate, X}}^{\anurg}=
%    \bigPchoiceOf{\anurg}_{t\in\transitions_{\astate, X}}\encoding{t}^{\anurg}\\
%    %
%    \encoding{\aterm\overset{\sigma|X}{\to}\atermp}^{\anurg}
%    &=\setvar{s_{\anurg}}{\astatep}\appl\encoding{\sigma}^{\anurg}\;\;
%    %
%    \encoding{\aterm\overset{\mathrm{nxt}}{\to}\atermp}^{\anurg}
%    =\setvar{s_{\anurg}}{\astatep}\appl\setvar{c_{\anurg}}{\mathrm{nxt}}\\
%    %
%    \encoding{\aterm\overset{\mathrm{new}}{\to}\atermp}^{\anurg}
%    &=\setvar{s_{\anurg}}{\astatep}\appl@\appl\$^{\anurg}\appl @
%\end{align*}
%
%
Using these elements, we encode the individual stacks 
as terms.
We say that $\aterm$ encodes 
$\stsymboln{0}...\stsymboln{k}\in\Gamma^{*}$
in urgency $\anurg$ if 
$\aterm=\stacksep\appl\atermp\appl\atermpp$ where 
$\atermp$ only contains terminals of urgency 
$\anurgp\geq\anurg$ with no assignments of $c_{\anurg}$, 
and removing all 
urgency $\anurgp>\anurg$ terminals from $\atermpp$ results in 
$\wrpsymboln{0}{\anurg}...\wrpsymboln{k}{\anurg}
\appl\wrplsymbol{\anurg}$.

The following lemma states the winning equivalence between 
encoding terms and encoded configurations.
\begin{lemma}\label{Lemma:LBoundSimulation}
    Let a player win $\aconfig=(\astate, 2\anurg - i, s_{0}, s_{1})$
    for some $\anurg\in\set{1, ..., \maxurg+1}$ and 
    $n\in\set{0, 1}$.
    If $\anurg=\maxurg+1$, then the player wins 
    the $\astate$-state term
    $\headerurg{\maxurg-1}
    \appl a\appl x_{1}$
    where $x_{1}$ encodes $s_{1}$ in urgency $\maxurg$.
    If $\anurg \leq \maxurg$, then the 
    player wins the $\astate$-state term 
    $\headerurg{\maxurg-1}\appl a\appl x_{0}\appl x_{1}$,
    where $x_{0}$ encodes $s_{0}$ in urgency $\anurg-i$
    and $x_{1}$ encodes $s_{1}$ in urgency $\anurg$.
\end{lemma}
